# Supplementary material for: XSS Vulnerabilities in Cloud-Application Add-Ons
Source: arXiv:1911.12332 source file (2019-11-27)
Supplement: Supplementary file 1 [file appendix.tex]

%!TEX root = ../main.tex
\appendix

\section{List of vulnerable add-ons}
\label{appendix:vulnerablelist}

\setcounter{table}{0}

\begin{table*}[tbh]
  \centering
  \caption{Vulnerable add-ons found in our study}
  \begin{tabular}{|l|p{5cm}|p{5cm}|}
    \hline
    \multirow{2}{*}{\textbf{Marketplace}} & \multicolumn{2}{c|}{\textbf{Vulnerable add-ons}}\\
    \cline{2-3}
    & \textbf{Popular} & \textbf{Randomly selected for analysis} \\ \hline

    Shopify & Order Printer Pro
            & ShipHero Fulfillment \newline
              Simple Admin \newline
              ShipRelay Fulfillment \newline
              Ship Systems 3D Box Packing \\ \hline
    MS Office Online & Translator for Outlook \newline
                    GIGRAPH - Network Visualization
                  & Duplicate Remover \newline
                    Bubbles \newline
                    Radial Bar Chart \newline
                    Excel to JSON \newline
                    WritingAssistant \newline
                    Excel to SMS
                  \\ \hline
    G Suite & formRanger \newline
              Flubaroo \newline
              autoCrat \newline
              formMule - Email Merge Utility \newline
              docAppender \newline
              Grackle Sheets \newline
              Sheetgo
            & Form Duplicates \newline
              Bulk Sheet Manager \newline
              rosterSync - Teacher Edition \newline
              Notifications for Forms \newline
              Text gBlaster (SMS Texting) \newline
              Mail Merge \newline
              Response Editor \newline
              Doc Variables \\ \hline

  \end{tabular}
  \label{tab:vulnerable_addons}
\end{table*}
